# Supplementary material for: Spin-polarized current in non-collinear antiferromagnets
Source: arXiv:1702.00295 ancillary file (2018-09-28)
Supplement: Supplementary file 1 [file supplemental_material.pdf]

# Supplemental Material

## 1 Calculation method

Here we include an in-depth description of the calculation method. We use a non-collinear DFT calculation to obtain the ground state band structure and wavefunctions denoted by $\varepsilon_{n\mathbf{k}}$ and $\varphi_{n\mathbf{k}}$ respectively. These could be directly used to evaluate Eq. 1 of the main text, however, in most cases this is very numerically demanding because a very dense k-mesh is needed for the evaluation of the sum. To make the calculation more tractable we use the so-called Wannier interpolation which enables us to efficiently calculate the band structure and wavefunctions for a subset of bands which lie close to the Fermi level. We first obtain the maximally localized Wannier functions (MLWFs) $w_{n\mathbf{R}}$ using the Wannier90 code [1, 2]. These are functions which satisfy for a set of $J$ bands

$$w_{n\mathbf{R}}(\mathbf{r}) = \frac{1}{N}\sum_{\mathbf{k}} e^{-i\mathbf{k}\cdot\mathbf{R}} \sum_{m=1}^{J} U^{\mathbf{k}}_{mn}\varphi_{m\mathbf{k}}. \tag{1}$$

$$\varphi_{n\mathbf{k}}(\mathbf{r}) = \sum_{\mathbf{R}} e^{i\mathbf{k}\cdot\mathbf{R}} \sum_{m=1}^{J} (U^{\mathbf{k}})^{-1}_{mn} w_{n\mathbf{R}}(\mathbf{r}).,\tag{2}$$

where $\mathbf{k}$ runs over all k-points in the first Brillouin zone, $\mathbf{R}$ runs over all Bravais lattice vectors and $U^{\mathbf{k}}$ are unitary matrices chosen so that the resulting Wannier functions are maximally localized. The transformation from the Bloch wavefunctions to the Wannier functions is a Fourier-like transformation.

Once the MLWFs are obtained we evaluate the Hamiltonian in the Wannier basis

$$H_{nm\mathbf{R}} = \langle n0|\,\hat{H}\,|m\mathbf{R}\rangle\,. \tag{3}$$

We can then Fourier transform this Hamiltonian to an arbitrary k-point:

$$\tilde{H}_{nm\mathbf{k}} = \sum_{\mathbf{R}} e^{i\mathbf{k}\cdot\mathbf{R}} H_{nm\mathbf{R}}. \tag{4}$$

This is the Hamiltonian written in the basis of functions

$$\tilde{\varphi}_{n\mathbf{k}}(\mathbf{r}) = \sum_{\mathbf{R}} e^{i\mathbf{k}\cdot\mathbf{R}} w_{n\mathbf{R}}(\mathbf{r}), \tag{5}$$

$$\tilde{H}_{nm\mathbf{k}} = \langle \tilde{\varphi}_{n\mathbf{k}}|\,H\,|\tilde{\varphi}_{m\mathbf{k}}\rangle\,. \tag{6}$$

By diagonalizing $\tilde{H}$ we obtain the band structure and the wavefunctions in the basis of $\tilde{\varphi}_{n\mathbf{k}}$. This method is quite efficient because the Hamiltonian $\tilde{H}_{nm\mathbf{k}}$ is relatively small as it contains only chosen number of bands that lie close to the Fermi level. Furthermore, since the Wannier functions are maximally localized, the matrix elements in Eq. (3) are large only for small $\mathbf{R}$ and thus we do not need a large mesh of $\mathbf{R}$ vectors.

If the energy window we are interested in does not contain an isolated set of bands (as is usually the case in metals) we have to choose from the bands contained in the energy window we are interested in a subset of $J$ bands which will be used to generate the Wannier functions. See [3] for the description of this method.

To evaluate Eq. 1 of the main text we also need the matrix elements of the velocity operator and of the spin current operator. The velocity operator is defined as

$$\hat{\mathbf{v}} = \frac{i}{\hbar}[\hat{H}, \hat{\mathbf{r}}], \tag{7}$$

where $\hat{\mathbf{r}}$ is the position operator. To evaluate the velocity operator we could thus first evaluate the position operator in the Wannier basis and then calculate the commutator with the Hamiltonian in the Wannier basis. In tight-binding calculations it is often assumed that the position operator is diagonal in the tight-binding basis. For simplicity we have also used this assumption, i.e., we assume that the position operator is diagonal in the Wannier basis. Then the velocity operator in the basis of functions $\tilde{\varphi}_{n\mathbf{k}}$ is given by

$$\hat{v}_{nm\mathbf{k}} = \frac{i}{\hbar}\sum_{\mathbf{R}} e^{i\mathbf{k}\cdot\mathbf{R}}(\mathbf{R} + \mathbf{r}_m - \mathbf{r}_n)H_{nm\mathbf{R}}, \tag{8}$$

where $\mathbf{r}_n$ are the Wannier centers. Note that for the velocity operator in this basis

$$\mathbf{v}_{nm\mathbf{k}} \neq \frac{1}{\hbar}\frac{\partial \tilde{H}_{nm\mathbf{k}}}{\partial \mathbf{k}}. \tag{9}$$

This relation would be satisfied if we would include the Wannier centers in the Fourrier transform in the following way

$$\tilde{\tilde{\varphi}}_{n\mathbf{k}} = \sum_{\mathbf{R}} e^{i\mathbf{k}\cdot(\mathbf{R}+\mathbf{r}_n)} w_{n\mathbf{R}}(\mathbf{r}) \tag{10}$$

(and analogously for the Fourier transform of the Hamiltonian). For the spin current operator we also need to evaluate the spin operator in the Wannier basis, which is straightforward in the Wannier90 code.

For obtaining the MLWFs we used a mesh of $8 \times 8 \times 8$ k-points. A similar number of $\mathbf{R}$ vectors is then used for the reverse transformation. For calculating the spin currents we use k-meshes between $100 \times 100 \times 100$ and $200 \times 200 \times 200$ k-points.

# 2 Symmetry of the spin conductivity tensors

In presence of spin-orbit coupling (SOC) the symmetry properties of the spin conductivity tensors can be analyzed using the method outlined in [4] for spin-orbit torque. Spin Hall conductivity tensors were also studied in a similar way in Ref. [5]. Using the transformation properties of the spin and velocity operators we can derive the transformation relations for the odd and even parts of the spin conductivity tensors. For a symmetry operation represented by a matrix $R$ we have

$$\sigma^{\text{odd}}_{ijk} = \det(R) R_{il} R_{jm} R^{-T}_{kn}\, \sigma^{\text{odd}}_{lmn}, \tag{11}$$

$$\sigma^{\text{even}}_{ijk} = \pm \det(R) R_{il} R_{jm} R^{-T}_{kn}\, \sigma^{\text{even}}_{lmn}, \tag{12}$$

where the plus sign refers to a unitary symmetry operation (i.e. symmetry operation that does not contain time-reversal), while the minus sign refers to an anti-unitary symmetry operation (i.e. containing time-reversal) and we use the Einstein summation notation. Note that by $R^{-T}$ we denote an inversion and transpose of a matrix $R$. In a cartesian coordinate system $R^{-T} = R$. These equations form a set of linear equations that have to be solved for each symmetry operation. For this we use the Linear-response-symmetry code, available at [6].

The resulting tensor for the odd spin conductivity are given in Table I of the main text. For completeness we give also the even spin conductivity tensors; see Table 1.

When SOC is ignored, the symmetry analysis becomes more complicated. This is because without SOC the spin is not coupled to the lattice directly. In a nonmagnetic system any pure

| | | no SOC | SOC |
|---|---|---|---|
| $Mn_3Sn$ | $\sigma^x$ | $\begin{pmatrix} 0 & 0 & 0 \\ 0 & 0 & 0 \\ 0 & 0 & 0 \end{pmatrix}$ | $\begin{pmatrix} 0 & 0 & 0 \\ 0 & 0 & \sigma^x_{yz} \\ 0 & \sigma^x_{zy} & 0 \end{pmatrix}$ |
| | $\sigma^y$ | $\begin{pmatrix} 0 & 0 & 0 \\ 0 & 0 & 0 \\ 0 & 0 & 0 \end{pmatrix}$ | $\begin{pmatrix} 0 & 0 & \sigma^y_{xz} \\ 0 & 0 & 0 \\ \sigma^y_{zx} & 0 & 0 \end{pmatrix}$ |
| | $\sigma^z$ | $\begin{pmatrix} 0 & \sigma^z_{xy} & 0 \\ -\sigma^z_{xy} & 0 & 0 \\ 0 & 0 & 0 \end{pmatrix}$ | $\begin{pmatrix} 0 & \sigma^z_{xy} & 0 \\ \sigma^z_{yx} & 0 & 0 \\ 0 & 0 & 0 \end{pmatrix}$ |
| $Mn_3Ir$ | $\sigma^x$ | $\begin{pmatrix} 0 & 0 & 0 \\ 0 & 0 & 0 \\ 0 & 0 & 0 \end{pmatrix}$ | $\begin{pmatrix} 0 & -\sigma^x_{xy} & \sigma^x_{xy} \\ \sigma^x_{yx} & -\sigma^x_{yy} & -\sigma^x_{yz} \\ -\sigma^x_{yx} & \sigma^x_{yz} & \sigma^x_{yy} \end{pmatrix}$ |
| | $\sigma^y$ | $\begin{pmatrix} 0 & 0 & 0 \\ 0 & 0 & 0 \\ 0 & 0 & 0 \end{pmatrix}$ | $\begin{pmatrix} \sigma^x_{yy} & -\sigma^x_{yx} & \sigma^x_{yz} \\ \sigma^x_{xy} & 0 & -\sigma^x_{xy} \\ -\sigma^x_{yz} & \sigma^x_{yx} & -\sigma^x_{yy} \end{pmatrix}$ |
| | $\sigma^z$ | $\begin{pmatrix} 0 & 0 & 0 \\ 0 & 0 & 0 \\ 0 & 0 & 0 \end{pmatrix}$ | $\begin{pmatrix} -\sigma^x_{yy} & -\sigma^x_{yz} & \sigma^x_{yx} \\ \sigma^x_{yz} & \sigma^x_{yy} & -\sigma^x_{yx} \\ -\sigma^x_{xy} & \sigma^x_{xy} & 0 \end{pmatrix}$ |

Table 1: The even spin conductivity tensors for $Mn_3Sn$ and $Mn_3Ir$.

spin rotation then becomes a symmetry of the system. In a magnetic system the spin is coupled to the magnetic order and we assume that the orientation of the magnetic order is fixed with respect to the lattice even without SOC. Thus in a magnetic system spin is indirectly coupled to the lattice through the magnetic order even without SOC. This is somewhat inconsistent since in an infinite crystal the orientation of the magnetic order is fixed by SOC. To resolve this inconsistency we can formally consider an infinitesimally small SOC which will fix the orientation of the magnetic order but will not influence the electronic structure in any other way. Thus the coupling of electron spin to the lattice does formally require SOC, however, it depends on SOC only indirectly and thus the effects generated by this coupling such as the spin currents discussed in this manuscript do not scale with the SOC strength. This is important since it means that such effects can be large also in systems which contain only light elements.

When a magnetic order is present some pure spin rotations will still be symmetries if they keep the magnetic order invariant. Furthermore some nonmagnetic symmetry operations will be a symmetry of the magnetic system when combined with a spin rotation, again if the combined symmetry operation leaves the magnetic order invariant. For example, in a coplanar magnetic system, 180 degree spin rotation around the axis perpendicular to the plane which contains the magnetic moments will flip the sign of all magnetic moments. Therefore, this spin rotation combined with a time-reversal symmetry operation will be a symmetry of any coplanar magnetic system in absence of SOC. As a consequence of this symmetry, there can be no AHE in a coplanar magnetic system without SOC. When the magnetic order is non-coplanar this symmetry is broken and there can in general be an AHE without SOC. Such AHE is known as the topological AHE and is mainly studied in skyrmions.

Note that we assume here that without SOC there are no orbital magnetic moments and thus the magnetic moments are purely due to spin. This is reasonable for most systems, however, in some systems an orbital magnetic moment can occur even without SOC [7]. Such orbital magnetic moment could change the symmetry of the system since orbital moments transform differently compared to the spin moments: the spin moments are rotated by the spin rotations while orbital moments are not.

If we now consider a symmetry composed of a normal symmetry operation $R$ and a spin

rotation $S$, then Eqs. (13), (14) can be generalized as

$$\sigma_{ijk}^{\text{odd}} = \det(R) S_{ip} R_{pl} R_{jm} R_{kn}^{-T} \sigma_{lmn}^{\text{odd}}, \quad (13)$$

$$\sigma_{ijk}^{\text{even}} = \pm \det(R) S_{ip} R_{pl} R_{jm} R_{kn}^{-T} \sigma_{lmn}^{\text{even}}, \quad (14)$$

since the spin rotation only influences the spin, which corresponds to the first coordinate of the spin conductivity tensor. These equations are no more difficult than the equations for the case with SOC. However, to the best of our knowledge, no classification of symmetry operations of magnetic systems in absence of SOC exists and furthermore the number of symmetry operations will be infinite in most systems. In the present work we have used a simple algorithm implemented also in the Linear-response-symmetry code, which generates a finite list of symmetries in absence of SOC for a given crystalline and magnetic structure. We can then proceed in the same way as in the case of SOC. The algorithm we have used is not guaranteed to produce a complete list of the symmetries, however, the agreement with numerical calculations shows that in the case of $Mn_3Sn$ and $Mn_3Ir$ there is no important symmetry operation missing. In the future a more systematic approach will have to be developed. The odd spin conductivity tensors without SOC obtained with this approach are given in Table I of the main text. The even spin conductivity tensors without SOC are given in Table 1. As we will show in a separate publication these are also in agreement with the numerical calculations.

## 3 Comparison with experimental resistivity

In Fig. 1 we plot the resistivity for $Mn_3Sn$ and $Mn_3Ir$ calculated using Eq. 1 of the main text as a function of $\Gamma$. The $\Gamma$ parameter describes the amount of disorder and thus we expect that it should roughly describe dependence of resistance on temperature since increasing the temperature increases the amount of disorder. The exact mapping of $\Gamma$ to temperature is, however, unclear. For $Mn_3Sn$ the experimental resistance at low temperatures is approximately 60 $\mu\Omega \cdot$cm for $\rho_{zz}$ and 80 $\mu\Omega \cdot$cm for $\rho_{xx}$ [8]. At room temperature the resistance is 480 $\mu\Omega \cdot$cm for $\rho_{zz}$ and 400 $\mu\Omega \cdot$cm for $\rho_{xx}$. In our calculation we also observe that $\rho_{xx}$ is larger than $\rho_{zz}$ for small $\Gamma$, while for larger $\Gamma$ $\rho_{xx}$ is smaller than $\rho_{zz}$. Furthermore we observer that for small $\Gamma$ the resistivity is increasing with $\Gamma$, while for large $\Gamma$ it is decreasing. This is also in agreement with the experiment. However, the value of resistivity in our calculation is clearly smaller than in the experiment. This is probably because the experimental samples contain a large amount of disorder; in particular the composition of the samples used in [8] is actually $Mn_{3.2}Sn$ and thus a significant chemical disorder is present.

For $Mn_3Ir$ the experimental resistivity at room temperature is $\rho_{xx} = 40$ $\mu\Omega \cdot$cm [9], this corresponds to $\Gamma \approx 0.05$ eV. For $Mn_3Ir$ we are not aware of any experimental measurement of the resisistivity dependence on temperature below room temperature and the resistivity does not show any interesting features like it does in the case of $Mn_3Sn$. Thus we cannot comment on the agreement of the calculated resistivity with the experiments. The fact that the calculated resistivity for $Mn_3Ir$ is significantly smaller than for $Mn_3Sn$ is at least in agreement with the experiment. Note, however, that in [10] a much larger resistivity is reported for $Mn_3Ir$ presumably because of large disorder being present.

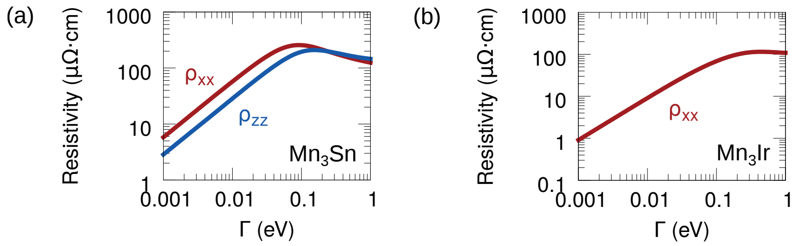


Figure 1: Calculated resistivity for (a) $Mn_3Sn$ and (b) $Mn_3Ir$ as a function of $\Gamma$.

## References


[1] N. Marzari and D. Vanderbilt, Phys. Rev. B **56**, 12847 (1997).

[2] A. A. Mostofi, J. R. Yates, G. Pizzi, Y.-S. Lee, I. Souza, D. Vanderbilt, and N. Marzari, Comput. Phys. Commun. **185**, 2309 (2014).

[3] I. Souza, N. Marzari, and D. Vanderbilt, Phys. Rev. B **65**, 035109 (2001).

[4] J. Železný, H. Gao, A. Manchon, F. Freimuth, Y. Mokrousov, J. Zemen, J. Mašek, J. Sinova, and T. Jungwirth, Phys. Rev. B **95**, 014403 (2017).

[5] M. Seemann, D. Ködderitzsch, S. Wimmer, and H. Ebert, Phys. Rev. B **92**, 155138 (2015).

[6] `https://bitbucket.org/zeleznyj/linear-response-symmetry`.

[7] J.-P. Hanke, F. Freimuth, S. Blügel, and Y. Mokrousov, ArXiv e-prints (2016), arXiv:`1610.07573`.

[8] S. Tomiyoshi, H. Yoshida, H. Ohmori, T. Kaneko, and H. Yamamoto, Journal of Magnetism and Magnetic Materials **70**, 247 (1987).

[9] T. Yamaoka, Journal of the Physical Society of Japan **36**, 445 (1974).

[10] W. Zhang, W. Han, S.-H. Yang, Y. Sun, Y. Zhang, B. Yan, and S. S. P. Parkin, Science Advances **2** (2016).
